# Supplementary material for: PI3D: Efficient Text-to-3D Generation with Pseudo-Image Diffusion
Source: arXiv:2312.09069 source file (2024-04-21)
Supplement: Supplementary file 1 [file X_suppl.tex]

\clearpage
\setcounter{page}{1}
% \maketitlesupplementary

% \appendix
% \section{More Results}
% \label{sec:diverse}
% We provide more 3D results, including diverse outcomes for the same text prompt.

\begin{figure*}[htbp]
    \centering
    \begin{overpic}[scale=0.2]{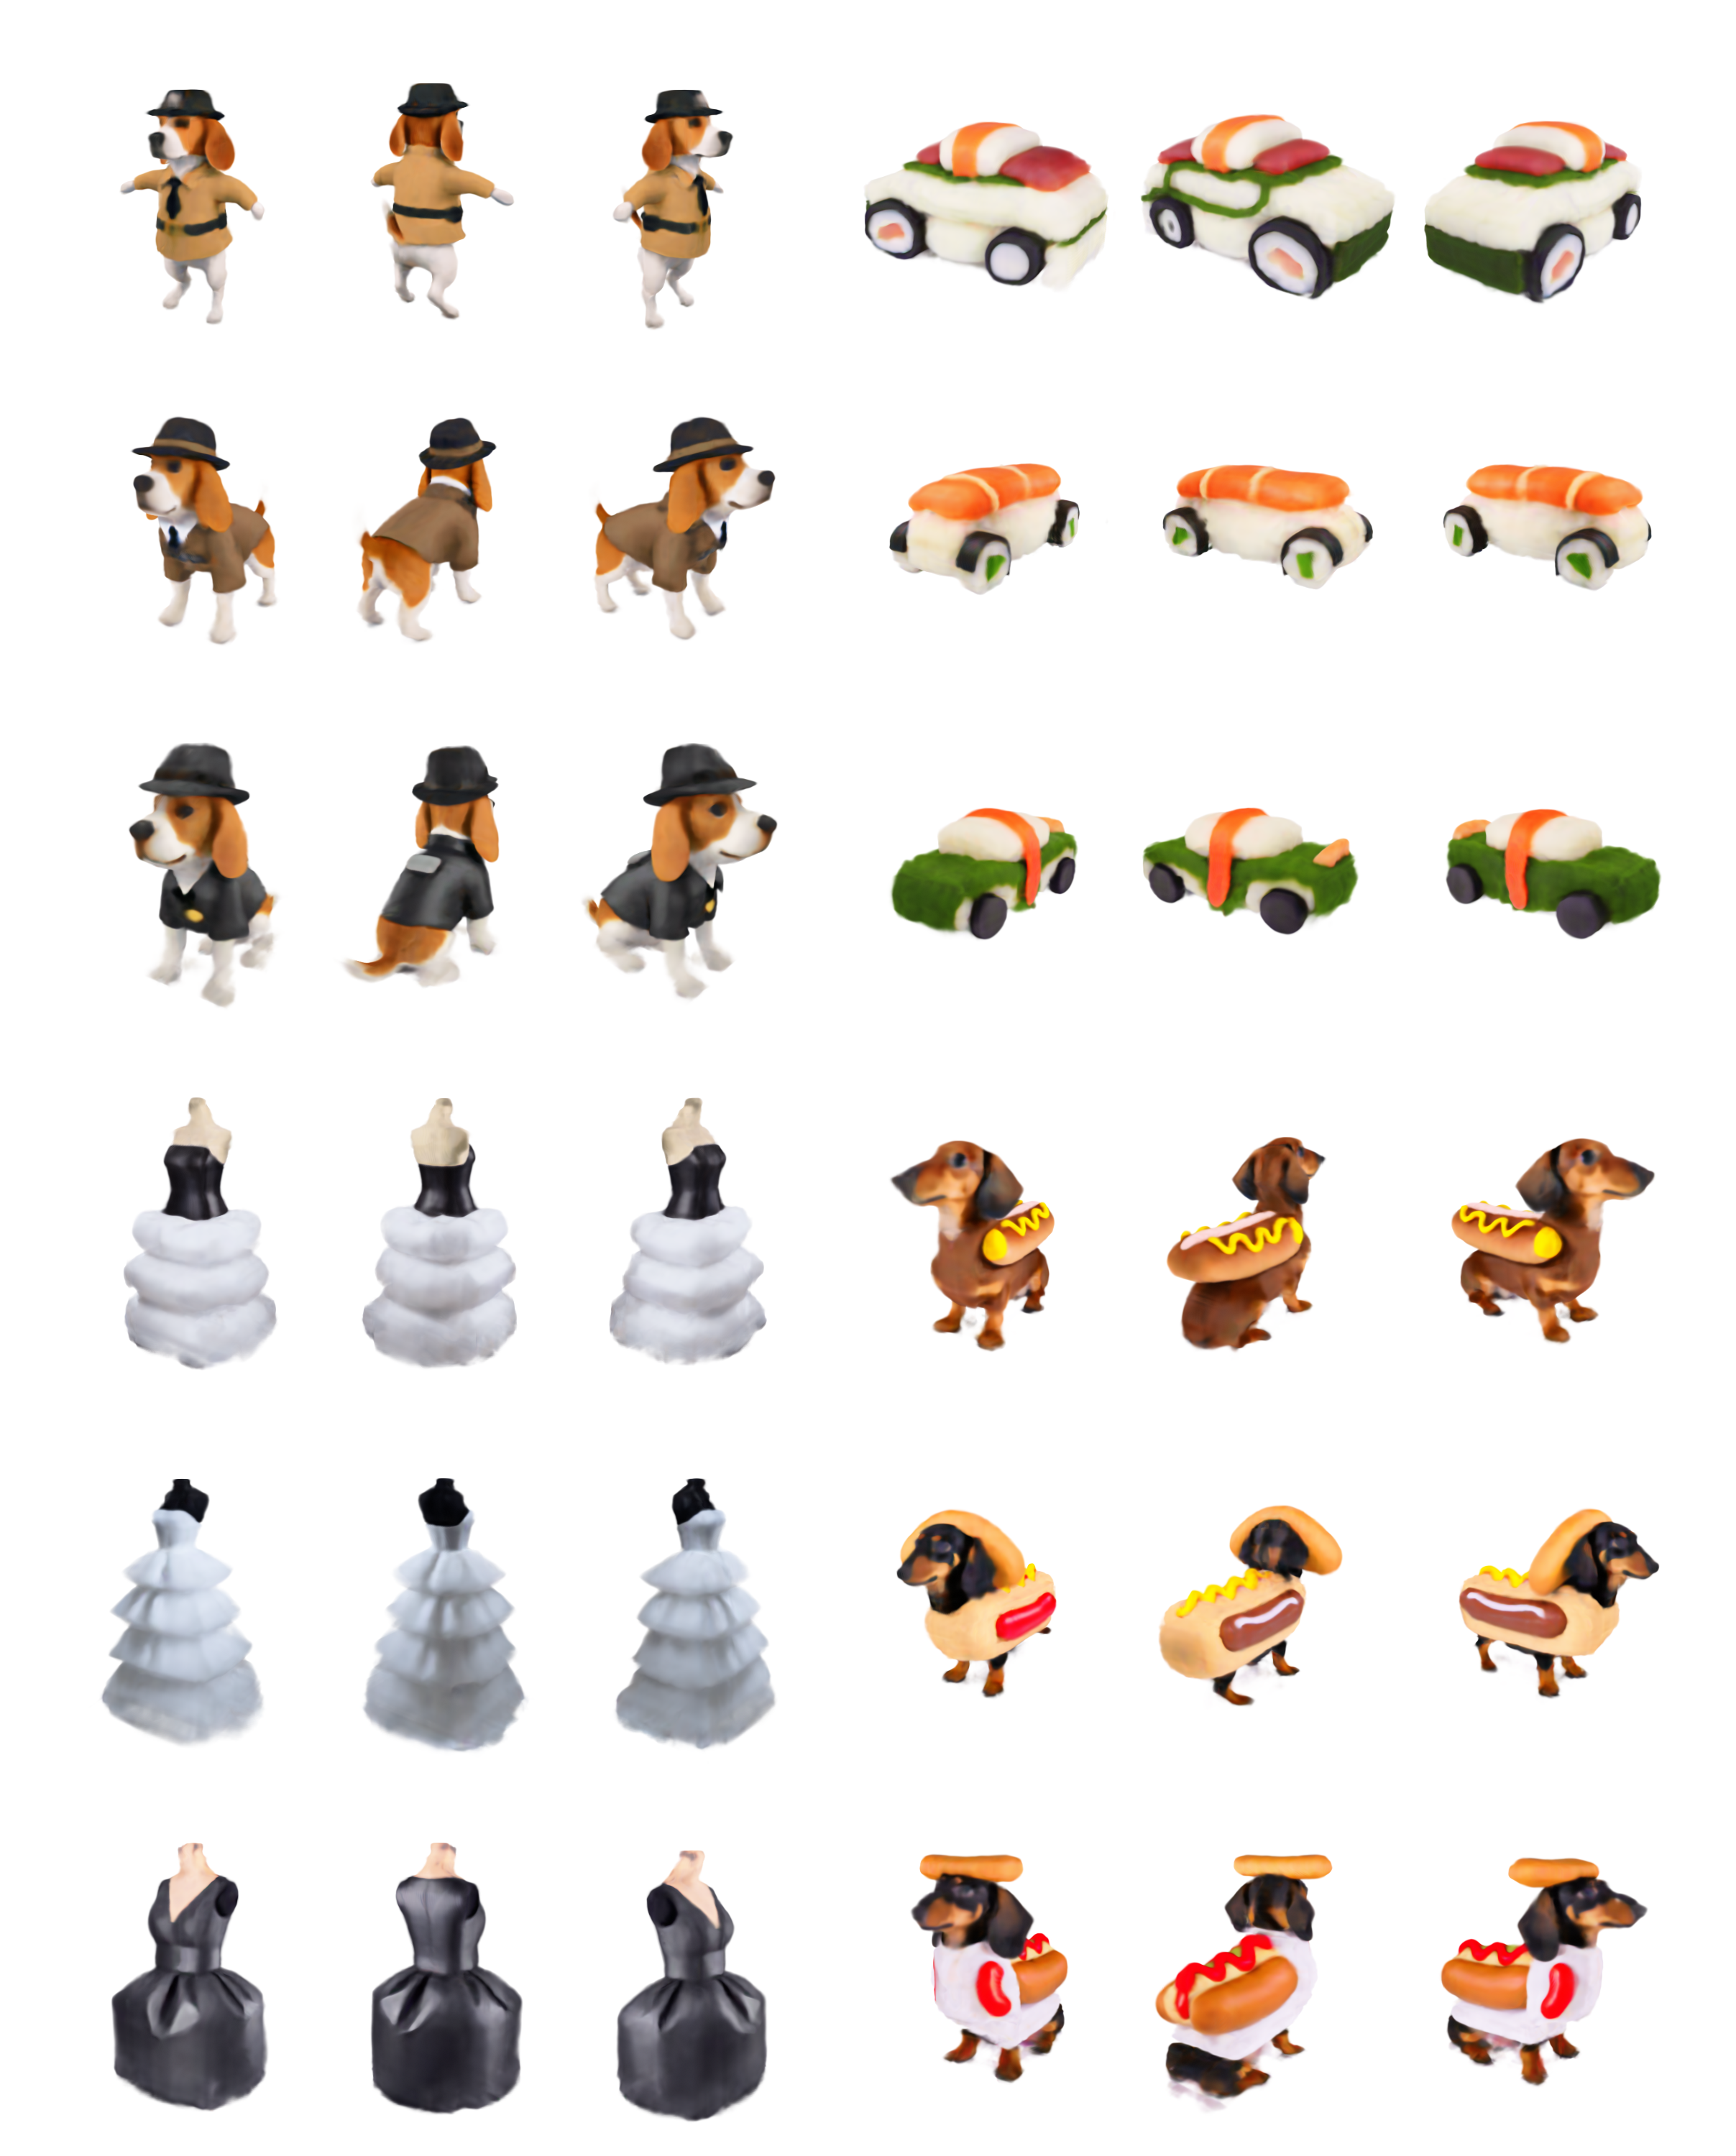}
    \put(70, 310){\textit{a beagle in a detective's outfit}}
    \put(0,0){\textit{a beautiful dress made out of garbage bags, on a mannequin}}
    \put(310,310){\textit{a car made out of sushi
    }}
    \put(270,0){\textit{a dachshund dressed up in a hotdog costume}}
    
    \end{overpic}
    \caption{We provide more generated results with diversity. We show 3 different outcomes for each text prompt.}
    \label{fig:supp1}
\end{figure*}

\begin{figure*}[htbp]
    \centering
    \begin{overpic}[scale=0.2]{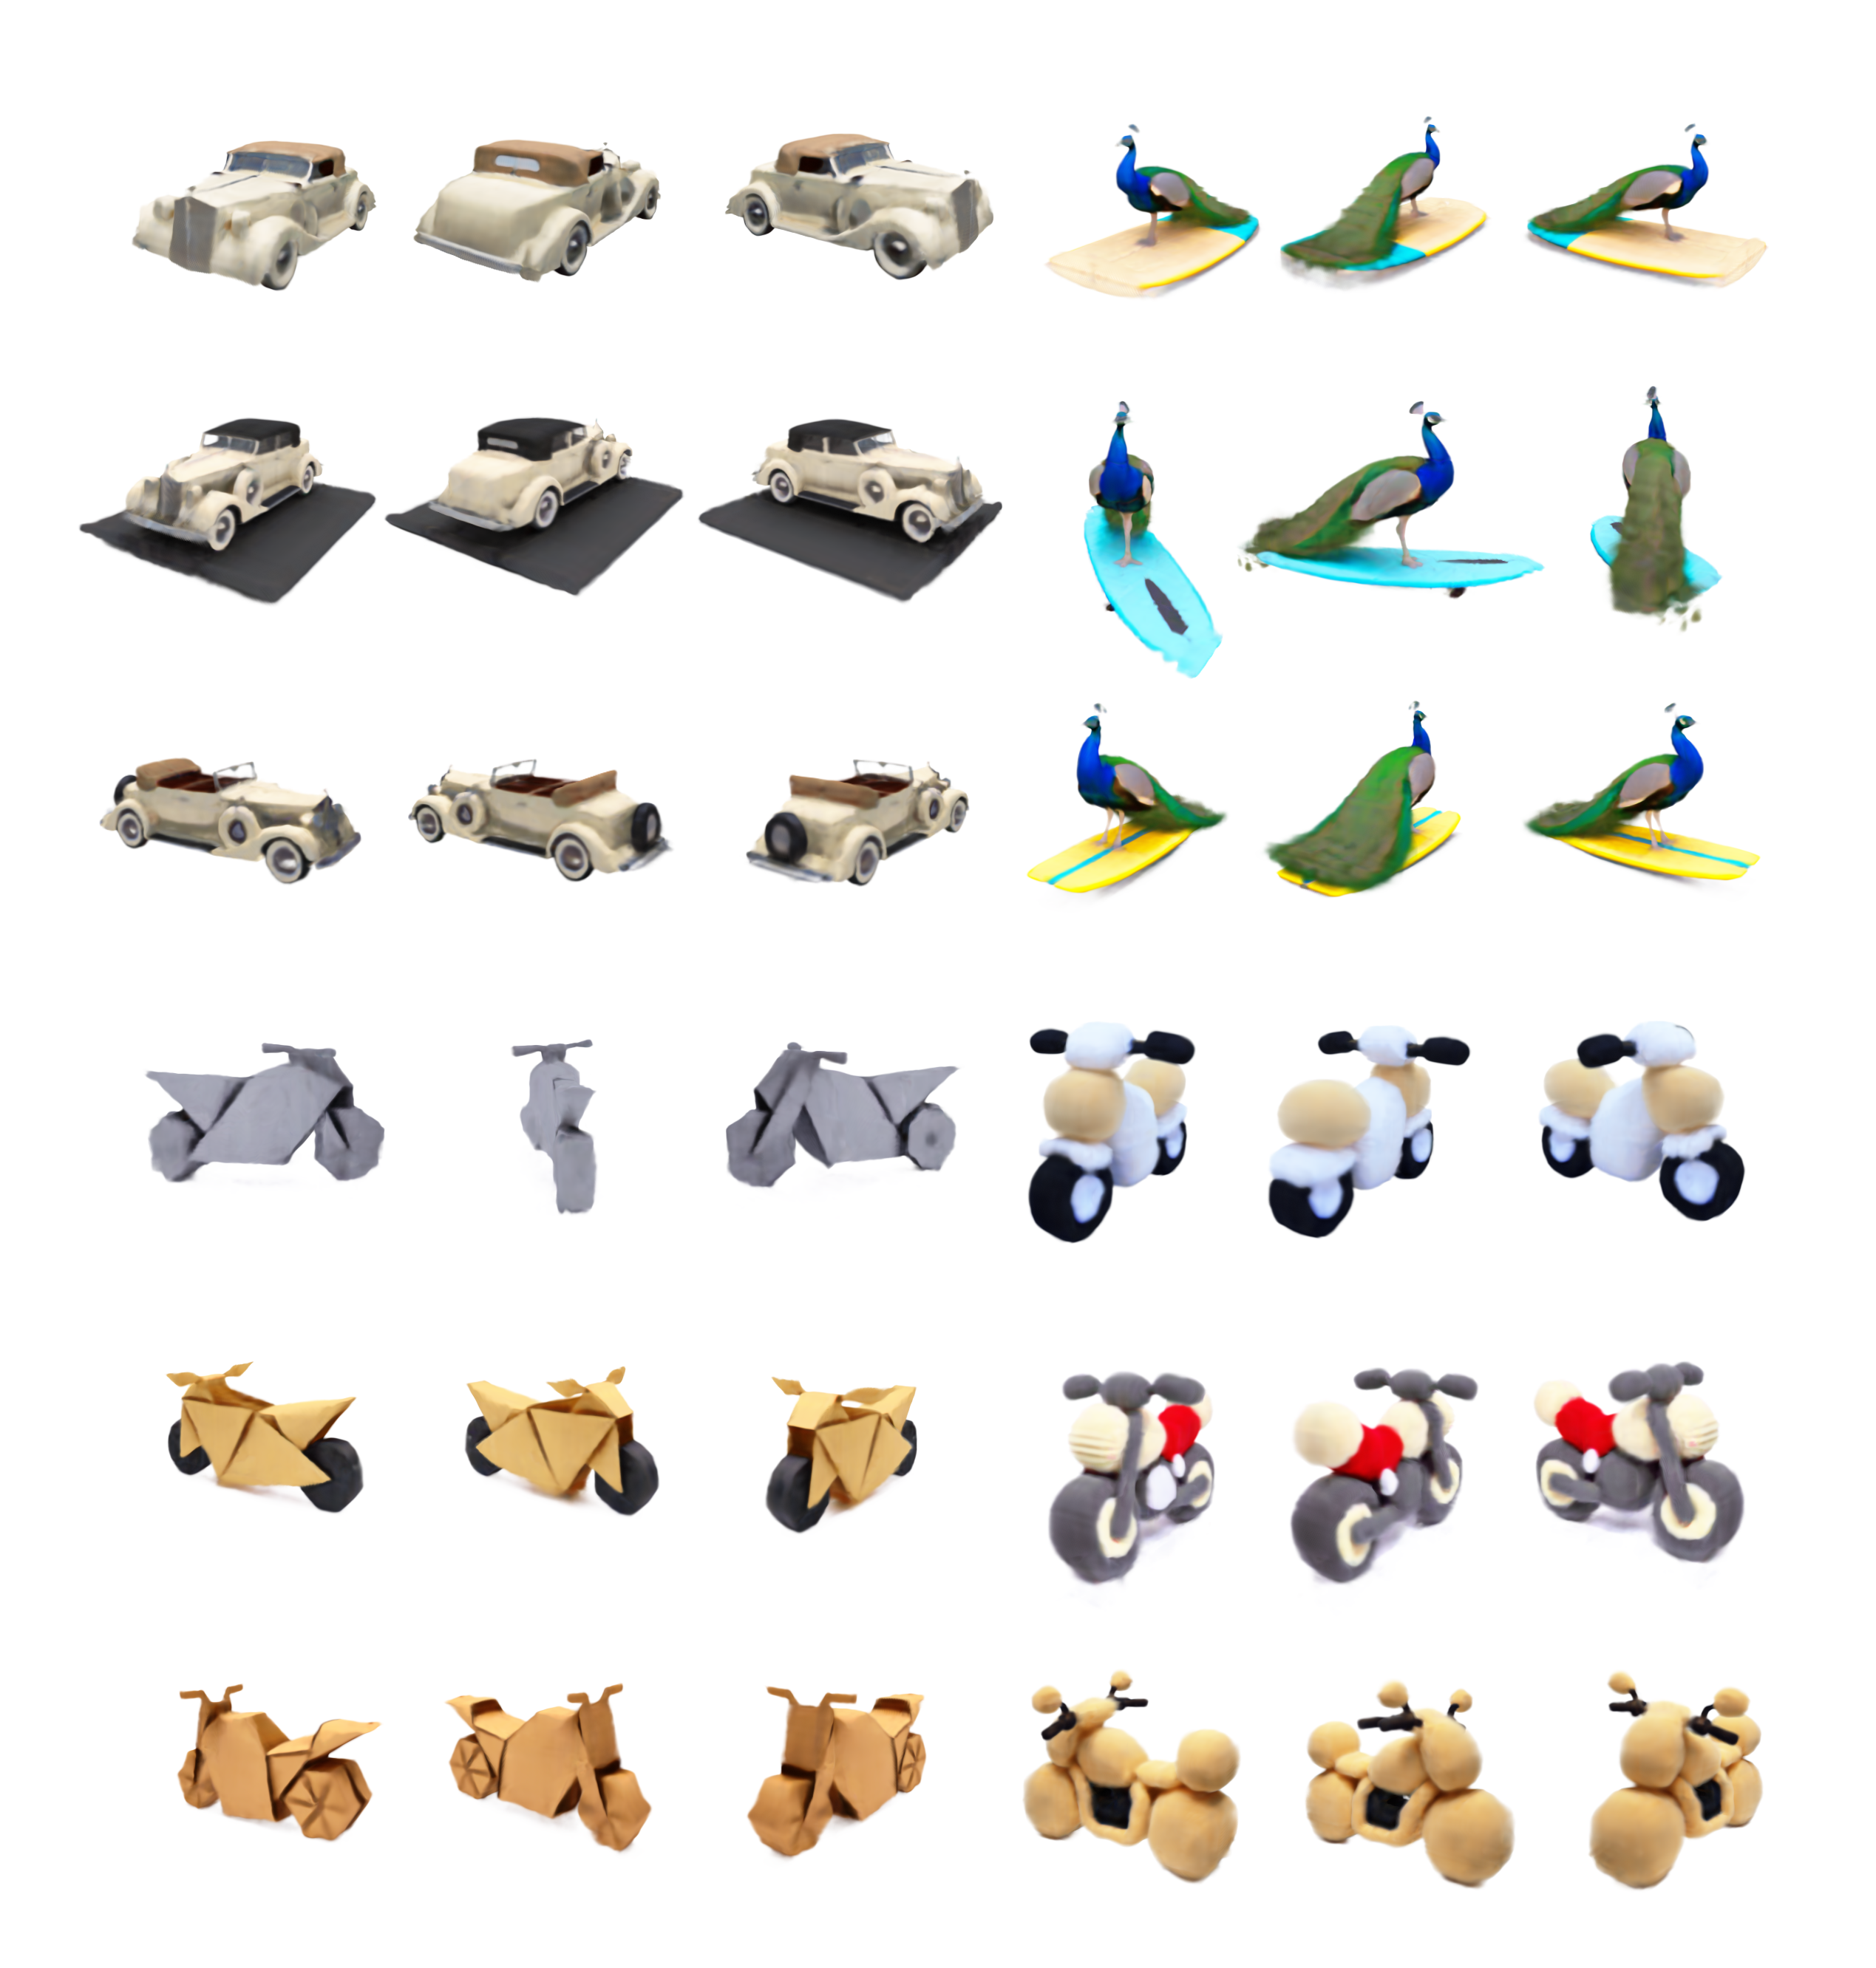}
    \put(330,270){\textit{a peacock on a surfboard}}
    \put(100,10){\textit{an origami motorcycle}}
    \put(330,10){\textit{an amigurumi motorcycle}}
    \put(100,270){\textit{a classic Packard car}}
    \end{overpic}
    \label{fig:supp2}
\end{figure*}

% % 
% Having the supplementary compiled together with the main paper means that:
% % 
% \begin{itemize}
% \item The supplementary can back-reference sections of the main paper, for example, we can refer to \cref{sec:intro};
% \item The main paper can forward reference sub-sections within the supplementary explicitly (e.g. referring to a particular experiment); 
% \item When submitted to arXiv, the supplementary will already included at the end of the paper.
% \end{itemize}
% % 
% To split the supplementary pages from the main paper, you can use \href{https://support.apple.com/en-ca/guide/preview/prvw11793/mac#:~:text=Delete%20a%20page%20from%20a,or%20choose%20Edit%20%3E%20Delete).}{Preview (on macOS)}, \href{https://www.adobe.com/acrobat/how-to/delete-pages-from-pdf.html#:~:text=Choose%20%E2%80%9CTools%E2%80%9D%20%3E%20%E2%80%9COrganize,or%20pages%20from%20the%20file.}{Adobe Acrobat} (on all OSs), as well as \href{https://superuser.com/questions/517986/is-it-possible-to-delete-some-pages-of-a-pdf-document}{command line tools}.
